# Supplementary material for: Simple biological controllers drive the evolution of soft modes
Source: arXiv:2507.11973 ancillary file (2025-07-16)
Supplement: Supplementary file 1 [file SI.pdf]

# Supporting Information

Christopher Joel Russo et al.

July 16, 2025

## 1 Simulations of Genetic Networks

### 1.1 In Silico Evolution of Non-Linear Gene Regulatory Network with a Simple Controller

As described in the main text, we model the gene regulatory network as a Michaelis-Menten network with an integral controller:

$$\frac{dn_a}{dt} = \sum_b k_{ab} \frac{n_b}{n_b + K_{ab}} - a_a s + \vec{\delta e}_{env} \tag{1}$$

$$s = c_p(\vec{s} \cdot \vec{\delta n}) + c_i \int (\vec{s} \cdot \vec{\delta n}) dt \tag{2}$$

where $n_a$ is the expression level of gene $a$ and $k_{ab}$ and $K_{ab}$ define the interactions between genes $a$ and $b$. The parameters $k_{ab}$ and $K_{ab}$ also determine the wild type fixed point. $\vec{s}, \vec{a}$ are parameters that determine the behavior of the controller and $\vec{\delta n}$ is $\vec{n}_{WT} - \vec{n}$, the deviation from the WT fixed point. We define a more *fit* system as having a lower absolute value of $\vec{\delta n}$, normalized by the overall stiffness of the system, averaged over many different values of $\vec{\delta e}_{env}$.

We simulate network evolution by selecting for higher fitness using a simulated annealing MCMC protocol (code available upon request). The interaction parameters $K_{ab}$ and $k_{ab}$ are initialized as random matrices with the following constraints: $k_{ab}$, $K_{ab}$ values are drawn from a uniform random distribution over [0,1] , with approximately 75% of entries set to zero to create sparse network structure. We ensure network stability at the wild-type fixed point by confirming that all eigenvalues of the Jacobian matrix have negative real parts before proceeding with simulations.

$\vec{s}, \vec{a}$ are constrained to be unit vectors, and are initially optimized for the starting $k_{ab}$ and $K_{ab}$ using the simulated annealing protocol. Then, $k_{ab}$ and $K_{ab}$ undergo evolution in the simulated annealing protocol. The Jacobian about the fixed point is computed at each simulated annealing time point about the fixed point for its $k_{ab}$ and $K_{ab}$, and the mode gap is calculated.

The model described by equations (1) and (2) represents a single-node controller ($k = 1$), where a single integral feedback mechanism operates on the system. This framework can be extended to multiple parallel controllers by increasing the number of controller nodes $k > 1$. For $k > 1$, each controller node i has its own sensing vector $\vec{s^i}$ and response vector $\vec{a^i}$ , allowing for more higher dimensional control strategies through multiple independent integral feedback mechanisms operating simultaneously. The generalized equations for $k > 1$ become:

$$\frac{dn_a}{dt} = \sum_b k_{ab} \frac{n_b}{n_b + K_{ab}} - \sum_k a_a^i s^i + \vec{\delta e}_{env} \tag{3}$$

$$s^i = c_p(\vec{s^i} \cdot \vec{\delta n}) + c_i \int (\vec{s^i} \cdot \vec{\delta n}) dt \tag{4}$$

At each cycle of the evolution simulation, we average over 5 evaluations of $\vec{\delta n}$ with different perturbations $\vec{\delta e}$ to assess fitness. The simulation employed simulated annealing with exponential cooling, with an initial temperature of $T_0 = 0.1$ and cooling rate $\alpha = 0.99$, for $\sim 1200$ steps. We run the evolution simulation for $k = 1$, and $k = 30$, the overall dimensionality of the system.

## 1.2 Simulation of Dual Buffering

We consider the same model of a gene regulatory network and controller with $k = 1$ nodes from above, reusing the $k_{ab}$ and $K_{ab}$ parameters with a slow mode, found via selection for robustness. Instead of environmental perturbations of the form $\vec{\delta e}_{env}$, we evaluate the fitness of the system as above, but with perturbations $\delta k_{ab}$ to the parameters of the interaction network, simulating mutation.

To implement perturbations to the interaction parameters, we add Gaussian noise with mean 0 and standard deviation 0.1 to a non-zero entry in the $k_{ab}$ matrix. This represents small mutations to the strength of interactions between genes. We then calculate how the steady-state expression levels change in response to these perturbations, both with and without the controller active. We quantify the fitness impact of mutations with and without the controller by measuring the average Euclidean distance between the perturbed and wild-type steady states. We plot the histograms of these effects in Figure 4b.

## 1.3 Simulation of Controller Knockout

To predict the impact on dimensionality of a controller knockout, we calculate the effect of the same ensemble of environmental perturbations as in section 1.1 with the controller as selected in section 1.1, and we also consider the same system but with the controller parameters set to 0. We compute PCA on the ensemble of effects $\delta x$ for both, showing dimensionality reduction when the controller is effectively knocked out (Figure 5a).

# 2 Linear Model of a Controller

## 2.1 Effective Rank

We can quantify the effective dimensionality of an ensemble of environmental perturbations $\{\vec{\delta e}_{env}\}$ using the effective rank metric [5] :

$$\text{rank}_{\text{eff}}(\{e_{env}\}) = \exp\Big( -\sum p_i \log(p_i)\Big) \tag{5}$$

where $p_i$ is the fraction of variance explained by the $i$th principal component. We can in the same way compute the effective rank of the ensemble of the **impacts** of these environmental perturbations $\text{rank}_{\text{eff}}(\{\vec{\delta x}\})$. We can show that it has the same effective rank as the ensemble of the environmental perturbations that caused them if all eigenvalues of $J_x$ are the same value, $\lambda$. Linearising the dynamics around the fixed point gives the map from perturbations to responses

$$\vec{\delta x} = J_x^{-1} \vec{\delta e}_{env}, \tag{6}$$

so the response covariance is

$$\Sigma_x = \langle \vec{\delta x} \vec{\delta x}^{\mathsf{T}} \rangle = J_x^{-1}\, \Sigma_e\, J_x^{-T}, \qquad \Sigma_e = \langle \vec{\delta e}_{env} \vec{\delta e}_{env}^{\mathsf{T}} \rangle. \tag{7}$$

If all eigenvalues of $J_x$ are equal, then $\Sigma_x = \lambda^{-2}\Sigma_e$. Because each PC variance is rescaled by the *same* factor $\lambda^{-2}$, the normalised spectrum is unchanged:

$$p_i^{(x)} = \frac{\lambda^{-2}\sigma_i^2}{\sum_j \lambda^{-2}\sigma_j^2} = p_i^{(e)}, \tag{8}$$

and therefore

$$\text{rank}_{\text{eff}}\big(\{\vec{\delta x}\}\big) = \text{rank}_{\text{eff}}\big(\{\vec{\delta e}_{env}\}\big)$$

This relationship holds because when all eigenvalues are identical, the system responds uniformly in all directions, preserving the dimensional structure of the input perturbations.

On the other hand, if the eigenvalues show a mode gap, (i.e. $\frac{\lambda_1}{\lambda_0} >> 1$), the effective rank $\text{rank}_{\text{eff}}(\{\vec{\delta x}\})$ can be *lower* than that of $\text{rank}_{\text{eff}}(\{\vec{\delta e}_{env}\})$. If we consider a system with a single slow mode $\lambda_0$ and all other modes $\lambda$, with a mode gap $\frac{\lambda}{\lambda_0}$ and a ensemble of perturbations where each entry $\delta e_{env,i} \sim N(0, \sigma)$. In the

eigenbasis of $J_x$, Eq. (7) yields response variances $\sigma^2/\lambda_0^2$ for the slow mode and $\sigma^2/\lambda^2$ for every fast mode. The normalized spectrum then becomes

$$p_0^{(x)} = \frac{(\lambda/\lambda_0)^2}{(\lambda/\lambda_0)^2 + (d-1)}, \qquad p_{i>0}^{(x)} = \frac{1}{(\lambda/\lambda_0)^2 + (d-1)}. \tag{9}$$

where $d$ is the number of dimensions of the system. Because $p_0^{(x)} \to 1$ while $p_{i>0}^{(x)} \to 0$ as $\lambda/\lambda_0 \to \infty$, the effective rank collapses:

$$\mathrm{rank}_{\mathrm{eff}}\big(\{\vec{\delta x}\}\big) \;\approx\; \exp\Big[-p_0^{(x)} \log p_0^{(x)} - (d-1) p_{i>0}^{(x)} \log p_{i>0}^{(x)}\Big] \ll \mathrm{rank}_{\mathrm{eff}}\big(\{\vec{\delta e}_{env}\}\big). \tag{10}$$

$$\mathrm{rank}_{\mathrm{eff}}(\{\vec{\delta e}_{env}\}) >> \mathrm{rank}_{\mathrm{eff}}(\{\vec{\delta x}\}) \tag{11}$$

The effective rank $\mathrm{rank}_{\mathrm{eff}}(\{\vec{\delta x}\})$ is greatly reduced from $\mathrm{rank}_{\mathrm{eff}}(\{\vec{\delta e}_{env}\})$ because the slow mode dominates the response - perturbations along this mode will cause much larger deviations in system state than perturbations in other directions. This creates a dimensional bottleneck that collapses the effective dimensionality of the system's responses compared to the dimensionality of the input perturbations.

## 2.2 General Model of a Controller and its Effectiveness Given an Arbitrary Perturbation

We consider a low-complexity integral feedback controller operating on system state $\vec{x}$, where $\vec{k}$ represents system parameters (including both external environmental parameters and internal interaction terms), and $f(\vec{x}, \vec{k})$ describes the uncontrolled system dynamics. The controller uses integral feedback with low complexity: a single sensing vector $\vec{s}$ compresses information about the system state into a one-dimensional scalar. The response vector $\vec{a}$ determines the direction along which the integral feedback acts to restore the system. The terms $k_i$ and $k_p$ represent the integral and proportional feedback gains, respectively.

$$\frac{d\vec{x}}{dt} = f(\vec{x}, \vec{k}) - \vec{a}\Big[k_p(\vec{s} \cdot \vec{\delta x}) + k_i \int (\vec{s} \cdot \vec{\delta x}) dt\Big] \tag{12}$$

We consider the linear regime about the fixed point. We refer to the uncontrolled effect of the perturbation as $\vec{\delta e}$

$$\frac{d\vec{x}}{dt} = f(\vec{x_0} + \vec{\delta x}, \vec{k_0} + \vec{\delta k}) - \vec{a}\Big[k_p(\vec{s} \cdot \vec{\delta x}) + k_i \int (\vec{s} \cdot \vec{\delta x}) dt\Big] \tag{13}$$

$$\approx \cancelto{0}{f(\vec{x_0}, \vec{k_0})} + J_x \vec{\delta x} + \cancelto{\vec{\delta e}}{J_k \vec{\delta k}} - \vec{a}\Big[k_p(\vec{s} \cdot \vec{\delta x}) + k_i \int (\vec{s} \cdot \vec{\delta x}) dt\Big] \tag{14}$$

$$\vec{\delta e} = J_x \vec{\delta x} + -\vec{a}\Big[k_p(\vec{s} \cdot \vec{\delta x}) + k_i \int (\vec{s} \cdot \vec{\delta x}) dt\Big] \tag{15}$$

Derive both sides

$$\frac{d\vec{\delta e}}{dt} = J_x \frac{d\vec{\delta x}}{dt} - \vec{a}\Big[k_p(\vec{s} \cdot \frac{d\vec{\delta x}}{dt}) + k_i(\vec{s} \cdot \vec{\delta x})\Big] \tag{16}$$

$$\cancelto{0}{\frac{d\vec{\delta e}}{dt}} = J_x \cancelto{0}{\frac{d\vec{\delta x}}{dt}} - \vec{a}\Big[k_p(\vec{s} \cdot \cancelto{0}{\frac{d\vec{\delta x}}{dt}}) + k_i(\vec{s} \cdot \vec{\delta x})\Big] \tag{17}$$

$$\vec{s} \cdot \vec{\delta x} = 0 \tag{18}$$

$$\vec{s} \cdot J_x^{-1} \vec{\delta e} = \cancelto{0}{\vec{s} \cdot \vec{\delta x}} - \vec{s} \cdot J_x^{-1} \vec{a}\Big[k_i \int (\vec{s} \cdot \vec{\delta x}) dt\Big] \tag{19}$$

$$(\sum s_i \vec{v_i}) \cdot \sum \frac{f_i \vec{v_i}}{\lambda_i} = -(\sum s_i \vec{v_i}) \cdot \sum \frac{g_i \vec{v_i}}{\lambda_i}\Big[k_i \int (\vec{s} \cdot \vec{\delta x}) dt\Big] \tag{20}$$

$$\sum \frac{s_i f_i}{\lambda_i} = -\sum \frac{g_i s_i}{\lambda_i}\Big[k_i \int (\vec{s} \cdot \vec{\delta x}) dt\Big] \tag{21}$$

$$I = \Big[k_i \int (\vec{s} \cdot \vec{\delta x}) dt\Big] = -\frac{\sum \frac{f_i s_i}{\lambda_i}}{\sum \frac{s_i g_i}{\lambda_i}} \tag{22}$$

Solving for $||\vec{\delta x}||^2$,

$$||\vec{\delta x}||^2 = ||\vec{\delta e} \oslash \vec{\lambda} - \left(\frac{\vec{\delta e} \oslash \vec{\lambda} \cdot \vec{s}}{\vec{a} \oslash \vec{\lambda} \cdot \vec{s}}\right) \vec{a} \oslash \vec{\lambda}||^2 \tag{23}$$

where $\vec{\lambda}$ is the vector of the eigenvalues of the Jacobian $J_x$.

## 2.3 Effectiveness of Controllers in Systems with a Slow Mode and Diverse Perturbations

We consider a system with one slow mode $\lambda_0$ and other modes of faster and equal $\lambda$. We assume that the perturbation $\vec{\delta e}$ is a random variable with $f_i \sim N(\mu_i, \sigma_i)$. We consider sensing and response unit vectors that operate along directions combining the mean perturbation direction $\hat{\mu}$ (excluding the slow mode) and the slow mode itself $\hat{v_0}$. The response vector is $\vec{a} = \beta \hat{v_0} + \sqrt{1-\beta^2} \hat{\mu}$ and the sensing vector is $\vec{s} = \alpha \hat{v_0} + \sqrt{1-\alpha^2} \hat{\mu}$. We find the expectation value of $||\vec{\delta x}||^2$

$$\begin{aligned}
\langle ||\vec{\delta x}||^2 \rangle &= \frac{1}{\lambda^2}\Big(\sum \mu_i^2 + \sigma_i^2\Big) \\
&+ \left(\frac{1}{\lambda_0^2} - \frac{1}{\lambda^2} + \Big(\frac{\lambda\alpha}{\lambda\alpha\beta + \lambda_0\sqrt{1-\alpha^2}\sqrt{1-\beta^2}}\Big)^2 \Big(\frac{\beta^2}{\lambda_0^2} + \frac{1-\beta^2}{\lambda^2}\Big) - 2\Big(\frac{\lambda\alpha}{\lambda\alpha\beta + \lambda_0\sqrt{1-\alpha^2}\sqrt{1-\beta^2}}\Big)\frac{\beta}{\lambda_0^2}\right)(\mu_0^2 + \sigma_0^2) \\
&+ \left(\Big(\frac{\lambda_0\sqrt{1-\alpha^2}}{\lambda\alpha\beta + \lambda_0\sqrt{1-\alpha^2}\sqrt{1-\beta^2}}\Big)^2 \Big(\frac{\beta^2}{\lambda_0^2} + \frac{1-\beta^2}{\lambda^2}\Big) - 2\Big(\frac{\lambda_0\sqrt{1-\alpha^2}}{\lambda\alpha\beta + \lambda_0\sqrt{1-\alpha^2}\sqrt{1-\beta^2}}\Big)\frac{\sqrt{1-\beta^2}}{\lambda^2}\right)\Big(\sum \mu_i^2 + \frac{\sum \mu_i^2 \sigma_i^2}{\sum \mu_j^2}\Big) \\
&\cdot \left(\frac{2\lambda\lambda_0\alpha\sqrt{1-\alpha^2}}{(\lambda\alpha\beta + \lambda_0\sqrt{1-\alpha^2}\sqrt{1-\beta^2})^2}\Big(\frac{\beta^2}{\lambda_0^2} + \frac{1-\beta^2}{\lambda^2}\Big) - \frac{2}{\lambda\alpha\beta + \lambda_0\sqrt{1-\alpha^2}\sqrt{1-\beta^2}}\Big(\frac{\alpha\sqrt{1-\beta^2}}{\lambda} + \frac{\beta\sqrt{1-\alpha^2}}{\lambda_0}\Big)\right)\Big(\mu_0 \sqrt{\sum_{j \neq 0} \mu_j^2}\Big)
\end{aligned} \tag{24}$$

We take the large $\lambda/\lambda_0$ limit, and find that optimal $\alpha, \beta = 1$ and this expression reduces to

$$\langle ||\vec{\delta x}|| \rangle = \frac{1}{\lambda} \langle ||\vec{\delta e}_{\perp \hat{v_0}}|| \rangle = \frac{1}{\lambda} \sqrt{\sum_{i \neq 0} (\mu_i^2 + \sigma_i^2)} \tag{25}$$

We can use this to derive a normalized effectiveness of the controller, dividing by the expected effect of a perturbation from this distribution in the absence of any control.

$$\langle ||\vec{\delta x}|| \rangle_{norm} = \frac{\sqrt{\sum_{i \neq 0} (\mu_i^2 + \sigma_i^2)}}{\sqrt{\sum_{i \neq 0} (\mu_i^2 + \sigma_i^2) + (\lambda/\lambda_0)^2 (\mu_0^2 + \sigma_0^2)}} \tag{26}$$

## 2.4 Fitness Benefit of Mode Gap with Varying Dimensionality

From the above equation, we can compute the benefit of increasing mode gap, say from $\lambda/\lambda_0 = 1$ to $\lambda/\lambda_0 = 100$ as a function of the dimensionality of the system.

$$\langle ||\vec{\delta x}|| \rangle_{\lambda/\lambda_0 = 1} - \langle ||\vec{\delta x}|| \rangle_{\lambda/\lambda_0 = 100} = \frac{\sqrt{\sum_{i \neq 0} (\mu_i^2 + \sigma_i^2)}}{\sqrt{\sum_{i \neq 0} (\mu_i^2 + \sigma_i^2) + (\mu_0^2 + \sigma_0^2)}} - \frac{\sqrt{\sum_{i \neq 0} (\mu_i^2 + \sigma_i^2)}}{\sqrt{\sum_{i \neq 0} (\mu_i^2 + \sigma_i^2) + (100)^2 (\mu_0^2 + \sigma_0^2)}} \tag{27}$$

To examine how this benefit scales with dimensionality, we consider a simplified case where $\mu_i = 0$ and $\sigma_i = \sigma$ for all $i$. In this case, as the dimensionality $n$ increases, the benefit of a mode gap approaches:

$$Benefit \approx \frac{\sqrt{(n-1)\sigma^2}}{\sqrt{(n-1)\sigma^2 + \sigma^2}} - \frac{\sqrt{(n-1)\sigma^2}}{\sqrt{(n-1)\sigma^2 + 10000\sigma^2}} = \frac{\sqrt{n-1}}{\sqrt{n}} - \frac{\sqrt{n-1}}{\sqrt{n-1+10000}} \approx \frac{\sqrt{n-1}}{\sqrt{n}} \tag{28}$$

This shows that as dimensionality increases, the benefit of having a mode gap approaches 1 (maximum possible benefit), and this approach is relatively rapid. Even in moderate dimensions (e.g., n=100), the benefit is approximately 0.9, indicating that the controller can eliminate nearly 90% of the perturbation effects.

# 3 High Throughput Yeast Fitness Data Analysis

## 3.1 Interaction Scoring

We apply the interaction scoring and significance testing methods from [1, 2]. Fitness is modeled as

$$f_{ij} = f_i f_j + e_{ij} \tag{29}$$

where $i, j$ are two mutations or a mutation and an environmental condition, $f_i$ is the single mutation/condition fitness, and $e_{ij}$ is the interaction between them. We use the "intermediate confidence" threshhold defined in the original papers, i.e. $P < 0.05$ and $|e| > 0.08$ to identify significant interactions between genes or genes and conditions.

For each gene pair or gene-condition pair, we use the $e_{ij}$ terms for each interaction as calculated in the original texts. The interaction score $e_{ij}$ represents the deviation from this expected value. Negative interaction scores are taken to indicate buffering.

We applied this analysis to both the gene-gene interaction data and the gene-environment interaction data to identify cases where genetic perturbations show significant interactions with either other genetic perturbations or environmental stresses.

# 4 Yeast Kinase Knockout Transciptomic Analysis

## 4.1 PCA on TPK123 Knockout vs. WT

We analyze the processed data from [4] – DESeq2 had been used to generate normalized expression values [3], and then the log2 fold change of each gene in each sample with respect to wild type cells in YPD was calculated. We conducted PCA on this data just Tpk123 knock-down and WT across conditions. To assess whether the controller knockout reduces dimensionality, we compared the eigenvalue spectra between the Tpk123 knock-down and wild-type conditions (see SFigure 1).

## 4.2 PCA Clustering

Using the same processed data from section 4.1, we repeat PCA, but on all knock-down experiments across all environmental conditions. To quantify the relative low dimensionality of the effects of environmental perturbations on Tpk123 knock-down cells, we quantify the mean euclidean distance between samples in different environmental conditions of a common genetic perturbation. We plot the histogram of the mean distance for all genetic perturbations, and highlight Tpk123 (Fig S1b).

For each knockdown-condition combination, we compute the mean Euclidean distance to all other knockouts within the same condition. We then average these distances across all conditions for each knockdown and plot the resulting histogram. (Fig S1c)

## 4.3 TSNE Clustering

As in section 4.2, we perform dimensionality reduction on all knock-down experiments across all environmental conditions, but with TSNE. We perform the same calculations as in 4.2, computing mean euclidean distance between samples in different environmental conditions of a common genetic perturbation and plotting its distribution (Fig5e), and computing the average of average intra-condition distances for each genetic perturbation and plotting its distribution (Fig5f).

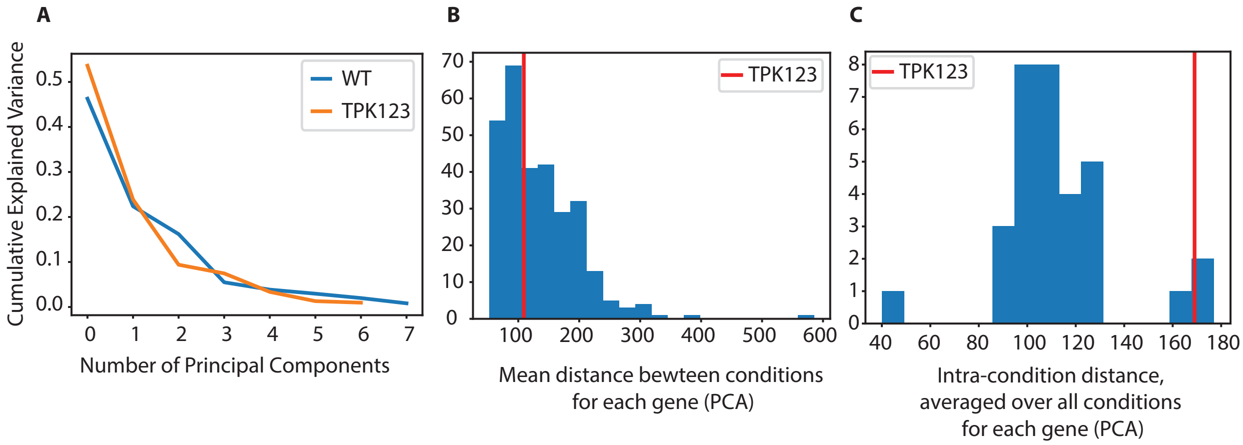


Figure 1: (a) We compute PCA on processed transcriptomic data for Tpk123 knock-down cells and WT cells across diverse environmental conditions. The bar plot shows the percentage of variance explained by each principal component. Note the dominant first principal component in the Tpk123 knockout data, indicating dimensionality reduction compared to wild-type.(b) The average distance in PCA space (first three components) to all other GxE samples of the same genetic background was computed and is plotted, and the TPK123 value is highlighted.

(c) The average distance in PCA space (first three components) to all other GxE samples of the same condition was computed, and then an average of averages was computed for each genetic background and is plotted. The TPK123 value is highlighted.

# References


[1] Michael Costanzo et al. "A global genetic interaction network maps a wiring diagram of cellular function". In: *Science* 353.6306 (2016), aaf1420.

[2] Michael Costanzo et al. "Environmental robustness of the global yeast genetic interaction network". In: *Science* 372.6542 (2021), eabf8424.

[3] Michael Love, Simon Anders, and Wolfgang Huber. "Differential analysis of count data–the DESeq2 package". In: *Genome Biol* 15.550 (2014), pp. 10–1186.

[4] Kieran Mace et al. "Multi-kinase control of environmental stress responsive transcription". In: *PLoS One* 15.3 (2020), e0230246.

[5] Olivier Roy and Martin Vetterli. "The effective rank: A measure of effective dimensionality". In: *2007 15th European signal processing conference*. IEEE. 2007, pp. 606–610.
